# Supplementary material for: Fermi surface topology and negative longitudinal magnetoresistance observed in centrosymmetric NbAs2 semimetal
Source: arXiv:1602.01795 source file (2016-03-14)
Supplement: Supplementary file 1 [file supplementalla.pdf]

# Supplementary material: Fermi surface topology and negative longitudinal magnetoresistance observed in $NbAs_2$ semimetal

Bing Shen,[1] Xiaoyu Deng,[2] Gabriel Kotliar,[2] and Ni Ni[1,*]

[1] *Department of Physics and Astronomy and California NanoSystems Institute, University of California, Los Angeles, CA 90095, USA*

[2] *Department of Physics and Astronomy, Rutgers University, Piscataway, NJ 08854, USA*

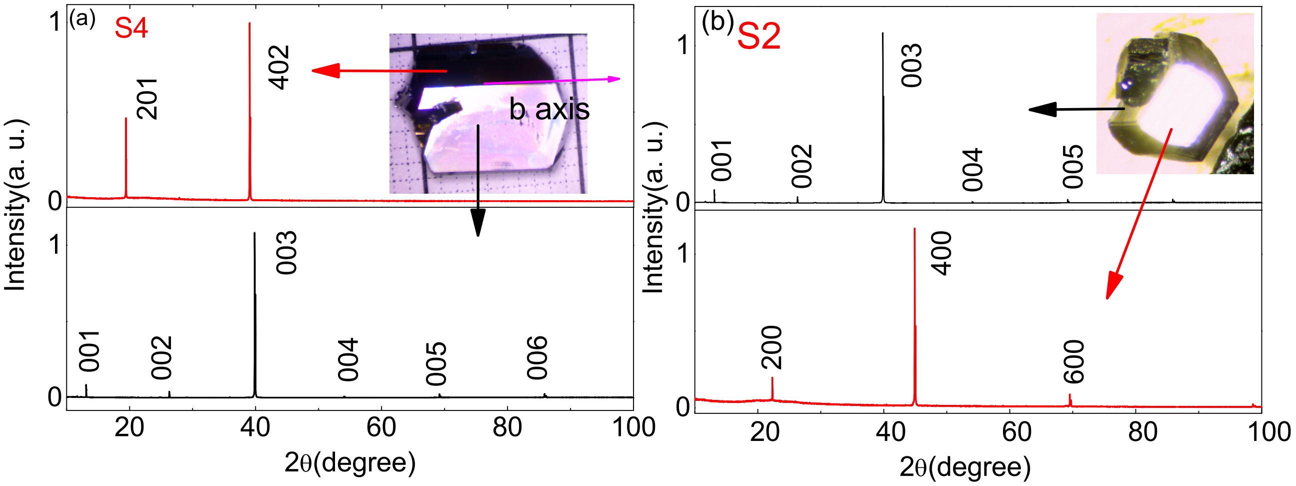


FIG. S1. The x-ray diffraction pattern for (a) sample S4 (b) sample S2. Insets: The pictures of single crystals of S4 (a) and S2 (b). The size of sample can be up to 10*8*3 mm$^3$.

**Single crystal growth and x-ray diffraction of $NbAs_2$**

Via the chemical vapor transport (CVT) method, single crystals of $NbAs_2$ were grown using $I_2$ as the transport agent during a two-week period. The source end was set at 950° and the sink end was held at 850°. The growth is endothermic and single crystals were found at the sink end. This is different from the CVT growth of NbAs which is exothermic. The growth habit of the majority of $NbAs_2$ single crystals were needle-like or blade-like with long direction along $b$ axis. Some of them are plate-like or even three dimensional. The size of the crystals was up to 10*8*3 mm$^3$, which could be shaped along different crystal axis. The crystal structure and crystal orientation were checked by x-ray diffraction and wavelength-dispersive spectroscopy (WDS) measurements. As representatives, x-ray diffraction patterns and the facets whic the x-ray diffractions were performedon are plotted in Fig. S1(a) for sample S4 and Fig. S1(b) for sample S2. The (0 0 1) and (2 0 1) planes of S2 were identified and the long shared edge between these two facets is thus determined to be along the $b$ axis. The top shinning facet of S4 was identified to be the (2 0 0) facet and the side plane was identified as the (0 0 1) facet. We then carefully shaped the S2 into a rectangular bar with the current along $a$ axis.

**The semiclassical two-band model fitting on $\rho_{xx}$ and $\rho_{yx}$**

Figure S2 (a) and (b) show representative $\rho_{xx}$ and $\rho_{yx}$ data of S1. The nonlinear Hall resistivity observed at 50 K indicates multiband effect in the system. To understand the mechanism of the large non-saturating transverse magneto-resistivity behavior, we used two band model to analyze our data. In the semiclassical two band isotropic model, the complex resistivity can be written as

$$\rho = \frac{1 + \mu\nu B^2 + i(\mu - \nu)B}{e(n\mu - p\nu) + i(p - n)\mu\nu} \tag{1}$$

Where n and p are carrier density for electron and hole, and the $\mu$ and $\nu$ are the mobility for electron and hole pockets. The transverse resistivity and hall resistivity can be acquired by $\rho_{xx}$=Re($\rho$) and $\rho_{yx}$=-Im($\rho$). We fit our data of $\rho_{xx}$ and $\rho_{yx}$ using these two formulas simultaneously and the fittings are shown in Fig. S2(a) and (b) as the red curves. The data are well fitted. The electron and hole are compensated and the electron-hole compensation behavior leads to the large TMR we observed. Table. S1 summarizes the $\mu$, $\nu$, $n$ and $p$ of different samples we measured and $NbAs_2$ samples in other groups. It is clear that the larger ratio of $R_{300K}/R_{2K}$ (RRR), the larger the transverse multiresistance TMR, consistent with the Kohler's law [1]. Obvious NLMR has been observed in both S2 and S4 whose RRR is 170 and 8000, respectively.

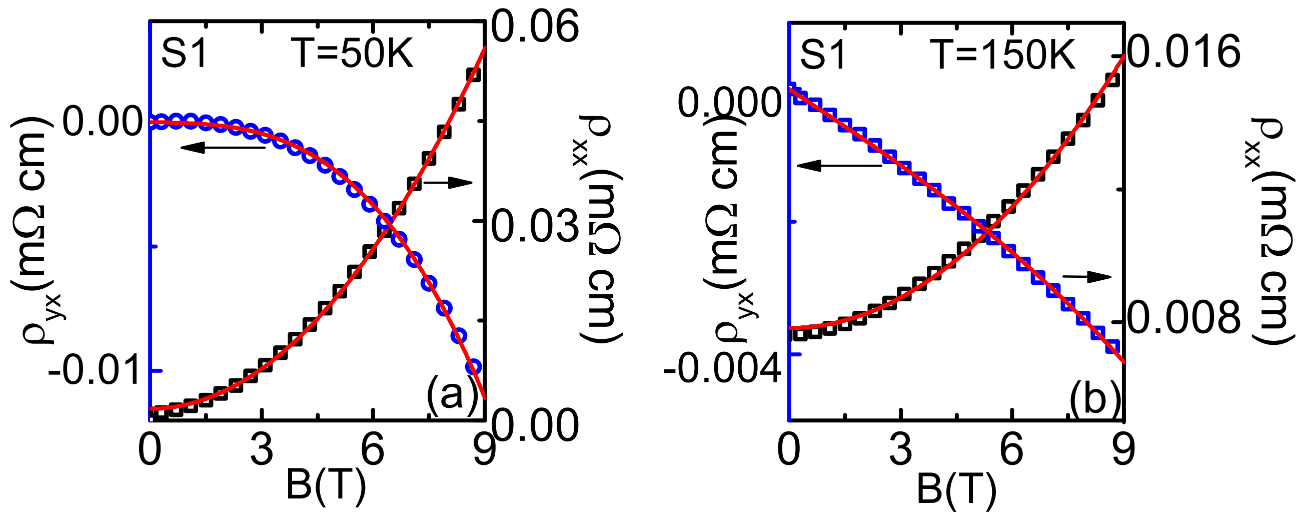


FIG. S2. (a) and (b): The temperature dependent resistivity, $\rho_{xx}$ (black) and Hall resistivity, $\rho_{xx}$ (blue) at 50 K and 150 K, respectively. Experimental data: symbols. Fitting: red curves.

TABLE S1. $n$, $p$, $\mu$, $\nu$, RRR and TMR of different $NbAs_2$ samples. The TMR of S1 to S4 was obtained at 1.8 K under 9 T while it was taken at 2.5 K under 14 T in ref. [2] and at 2 K under 9 T in ref. [3].

| | n ($10^{26}/cm^3$) | p ($10^{26}/cm^3$) | $\mu$($m^2V^{-1}S^{-1}$) | $\nu$($m^2V^{-1}S^{-1}$) | RRR | TMR |
|---|---|---|---|---|---|---|
| S1 | 4.1 | 3.9 | 1.9 | 1.4 | 37 | 230 |
| S2 | 1.1 | 1.1 | 1.5 | 1 | 34 | 170 |
| S3 | 4.8 | 4.6 | 1.0 | 0.9 | 35 | 143 |
| S4 | 0.18 | 0.18 | 2 | 1.9 | 222 | 8000 |
| $NbAs_2$ [2] | | | | | | 1000 |
| $NbAs_2$ [3] | 0.17 | 0.15 | 10 | 40 | 317 | 8800 |

**The data analysis of angular-dependent SdH**

To investigate the Fermi surface topology, we performed SdH quantum oscillation measurements. Three frequency peaks were observed in the FFT spectrum of $\Delta\rho_{xx}$. To get the information for each Fermi pocket, we adopted different filter to separate each oscillation. We applied a pass FFT filter (96 T<F< 148 T) to extract the oscillation pattern associated with the frequency $F_b$ (122 T) as shown Fig. S3 (b). Using similar procedures, we got the oscillation patterns associated with $F_a$ (227 T) and $F_c$ (76 T) with the pass FFT filter of 188 T<F< 288 T for $F_a$ and 10 T<F< 96 T for $F_c$, respectively. By summing these three individual oscillation patterns, we reconstructed the total $\Delta\rho_{xx}$. Figure. S3(a) shows the reconstructed $\Delta\rho_{xx}$ with $1/B$ ranging from 0.19 to 0.30. In the main text, Fig. 2(a) shows the reconstructed $\Delta\rho_{xx}$ with $1/B$ varying from 0.11 to 0.19. It is clear that the experimental data and reconstructed patterns match well. The subtle difference between these two above 0.26 may comes from the the excluded higher-frequency component.

Based on the respective $\delta\rho_{xx}$ associated with $F_b$ taken at different temperatures, at $B$=8.3 T, we got temperature dependent normalized amplitude, as shown in Fig. S3(c). Using the Lifshits-Kosevich (LK) formula with $B$=8.3 T, we obtained $m_b^* = 0.24(1)m_e$. We did the same procedure with $B$=7.3, we obtained $m_b^* = 0.23(1)m_e$. Based on the $\delta\rho_{xx}$ associated with $F_b$ taken at 1.8 K, we obtained field dependent normalized amplitude, as shown in Fig. S3(d). By fitting the field dependent amplitudes at 1.8 K, we obtained Dingle temperature as $T_D^b$=3.4 K. Using similar procedures, we determined the effective mass and Dingle temperature associated with $F_a$ and $F_c$.

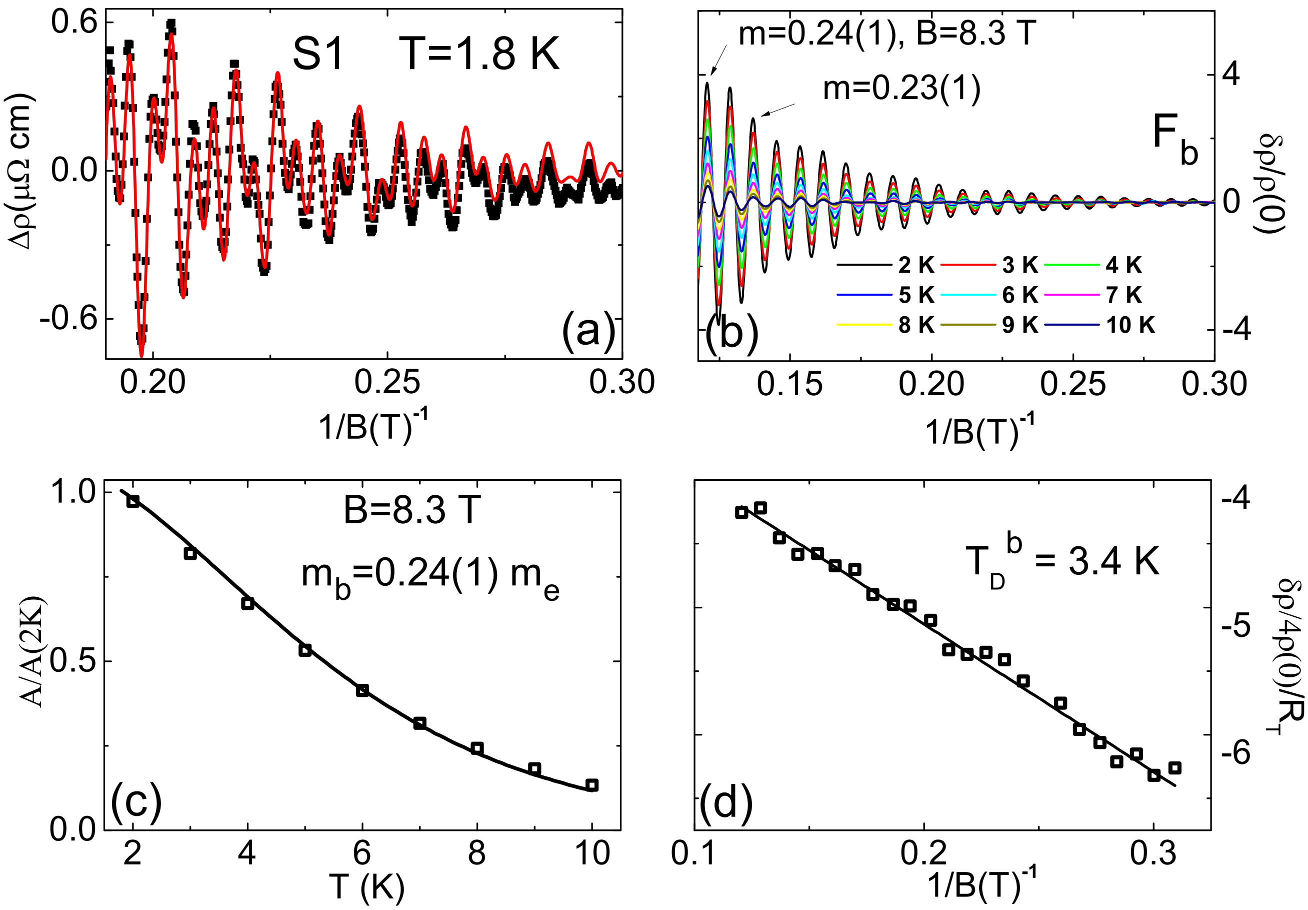


FIG. S3. (a) The total oscillation $\Delta\rho_{xx}$ vs $1/B$ measured at 1.8 K with $1/B$ from 0.19 to 0.30 ($\mathrm{T}^{-1}$). Experimental data (dots); Reconstructed curve (line). (b) The reconstructed oscillation $\delta\rho_{xx}$ originating from $F_a$ using inverse FFT. (c) The normalized temperature dependent amplitude of the respective $\delta\rho_{xx}$ associated with $F_b$. Solid line: fitting. (d) The Dingle plots of the respective $\delta\rho_{xx}$ associated with $F_b$. Solid lines: fitting. $\rho_0$ is the residual resistivity at 0 T and $R_T = \frac{\alpha T m^*/B}{sinh(\alpha T m^*/B)}$.

**Band structure, Fermi surface and the Brillouin zone folding effects**

We have performed first-principles calculations for $NbAs_2$ with two different setups shown in Fig. S4(a): (I) using the primitive cell structure with two formula of $NbAs_2$ (red edges) and (II) using the conventional cell structure with four formula of $NbAs_2$ (black edges). In both cases, we have obtained very similar results. We find that it is very instructive to understand the various experimental setups in the centered monoclinic structure by starting from the simpler Brillouin Zone (BZ) of the conventional cell. Therefore for the sake of better illustration, we choose to show the results from the latter setup in the main text. Here we provide band structure and Fermi surfaces for the primitive cell setup.

As expected in the conventional cell setup, bands and Fermi surfaces are folded from the larger BZ of the primitive cell into the smaller BZ of the corresponding conventional cell. Since this folding process is beneficial to understand various properties considering the electronic structure, we illustrate the process in Fig. S4(b), where the first BZs of the primitive cell (red dashed line) and the conventional cell (black solid line) are depicted together.

We plot the band structure of the primitive cell setup in Fig. S4(c). For comparison the band structure for the conventional cell is plotted side by side (Fig. S4(d)). From Fig. S4(b), it is clear that M and A points in Fig. S4(c) are folded to X point in Fig. S4(d). Therefore the band crossings near X point (inset of Fig. S4(d)) are simply the effects arising from the BZ folding, thus are not gapped by spin-orbit coupling.

The Fermi surface of the primitive cell is computed using in total 200000 k-point in the BZ, and is shown in Fig. S4(e). The results are consistent with those computed in the conventional cell as shown in the main text. In total

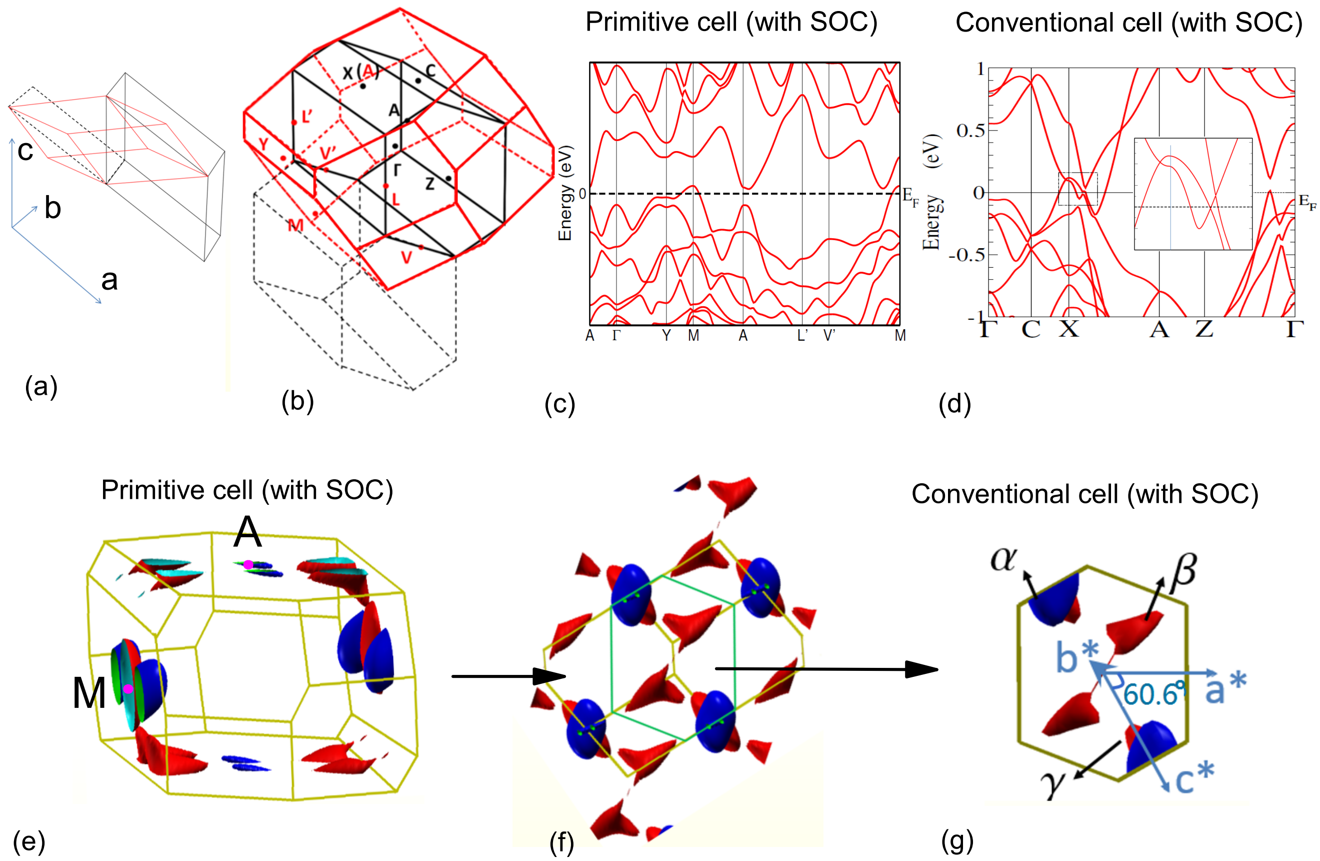


FIG. S4. (a) The chosen unit cell of $NbAs_2$ in the conventional cell setup (black) and the primitive cell setup (red) in the calculations. (b) The corresponding first Brillouin zone (BZ) of the conventional cell setup (black) and the primitive cell (red). High symmetry points of the BZ zones of the conventional cell (black letters) and the primitive cell (red letters) are labeled. (c) The band structure of $NbAs_2$ in the primitive cell setup. (d) The band structure of $NbAs_2$ in the conventional cell setup. (e) The Fermi surfaces of $NbAs_2$ shown in the first BZ of the primitive cell. (g) The top view (along $b^*$ axis) of the Fermi surfaces as in (e), expanded periodically in momentum space. The light-green lines denote the corresponding BZ of the conventional cell. (f) The top view of the Fermi surfaces in the BZ of the conventional cell.

we have found mainly four types of Fermi surfaces. We note a dense k-mesh is necessary to capture the small $\delta$ sheet satisfactorily. From Fig. S4(b), it is seen that the $\gamma$ sheet overlaps with the $\delta$ sheet in the BZ of the conventional cell due to BZ folding, consistent with the inset of Fig. S4(d). A schematic illustration of the folding process is shown in Fig. S4(f), in which the BZ of the primitive cell is expanded periodically in momentum space. By viewing along the $b^*$ axis, we obtain the same pattern as shown in Fig. S4(g) which is obtained with the conventional cell set up. In addition, for both setups, we have tried to extract the quantum oscillation frequency using SKEAF, and have obtained consistent results. We extract the frequency for the $\delta$ sheet in the primitive setup only to avoid its overlap with $\gamma$ sheet due to BZ folding.

* Corresponding author: nini@physics.ucla.edu

[1] A. B. Pippard, Magnetoresistance in metals, (Cambridge University Press,Cambridge, 1984).
[2] Y.-Y. Wang, Q.-H. Yu, T.-L. Xia, Unpublished, arXiv:1601.04239 (2016).
[3] Z. J. Yuan, H. Lu, Y. J. Liu, J. F. Wang, S. Jia, Unpublished, arXiv:1601.06482 (2016).
[4] D. Shoenberg, Magnetic oscillations in metals, (Cambridge, University Press,Cambridge, 1984).
